# Supplementary material for: MoS$_{2}$ nanosheets incorporated {\alpha}-Fe$_{2}$O$_{3}$/ZnO nanocomposite with enhanced photocatalytic dye degradation and hydrogen production ability
Source: arXiv:2111.07185 source file (2021-11-13)
Supplement: Supplementary file 1 [file appendix1.tex]

\section{Supplementary Material} \label{sec:appendix}
    Here the ESI will be included.
